# Supplementary material for: A Comparative Exploration of ML Techniques for Tuning Query Degree of Parallelism
Source: arXiv:2005.08439 source file (2020-05-21)
Supplement: Supplementary file 1 [file appendix.tex]

\section{Appendix}
